# Supplementary material for: RoboWorM: Evaluating Movement Realism, Consistency and Acceleration Affects in Embodied Video World Models
Source: arXiv:2610.33807 source file (2026-10-24)
Supplement: Supplementary file 2 [file 6_kiva.tex]

\section{KIVA Implementation Details}
\label{supp:kiva}

\subsection{Coordinate Representation and Reader Architecture}
\label{supp:kiva_reader}

\paragraph{Ground-truth coordinates.}
Training targets are computed from recorded robot states through
robot-specific forward kinematics, including gripper opening when needed to
locate finger keypoints. For robots with end-effector pose logs rather than
joint-angle logs, keypoints are constructed from the recorded pose and gripper
opening. All coordinates are expressed in the robot base frame, in meters.

\paragraph{Workspace normalization.}
Let $X_{\min}$ and $X_{\max}$ denote coordinate-wise extrema over the training
keypoints, and let $a=X_{\max}-X_{\min}$. We fit a workspace box with a $5\%$
margin on each axis:
\begin{equation}
\ell=X_{\min}-0.05a,
\qquad
h=X_{\max}+0.05a.
\end{equation}
Metric coordinates are normalized and recovered through
\begin{equation}\label{eq:supp-norm}
\begin{aligned}
E(X) &= 2(X-\ell)\oslash(h-\ell)-1,\\
E^{-1}(x) &= (x+1)\odot\frac{h-\ell}{2}+\ell,
\end{aligned}
\end{equation}
where $\oslash$ and $\odot$ denote coordinate-wise division and multiplication.
The workspace spans $h-\ell$ must be positive on all axes. The box is fitted
only on training data and retained unchanged for inference. The clean training
target is $x_0=E(X^{\mathrm{FK}})$, where $X^{\mathrm{FK}}$ are the
forward-kinematics coordinates in meters.

\paragraph{Visual features.}
Each camera view is resized to $768\times768$ and normalized using ImageNet
statistics before encoding with a frozen DINOv3 ViT-L/16. We discard class and
register tokens and apply non-overlapping $2\times2$ average pooling to the
$48\times48$ patch grid. Concatenating the resulting tokens from $V$ views gives
$\mathcal F_\tau\in\mathbb R^{576V\times1024}$. The encoder remains frozen and
its features are cached during training.

\paragraph{Denoising head.}
The coordinate embedding $\phi$ in Eq.~\eqref{eq:head} applies ten
Fourier-frequency bands followed by an MLP, while the noise embedding $\psi$
uses sinusoidal features followed by an MLP. Learned embeddings identify
keypoints ($e_k$), camera views, spatial patch positions, and temporal
positions ($p_{1:T}$).

The cross-attention module $\operatorname{CA}$ comprises two cross-attention
blocks and an output normalization layer; each keypoint query attends to visual
tokens from its own frame only. The temporal module $\operatorname{TA}$
comprises four bidirectional Transformer encoder layers, applied separately to
each keypoint track, so information is shared across time but not across
keypoints. Both modules use hidden width 512, eight attention heads,
feed-forward width 2048, and dropout 0.1.

Visual keys and values are shared across the two cross-attention blocks and
reused across denoising steps and samples. The output projection
$W_{\mathrm{out}}$ is shared across keypoints, with weights and bias initialized
to zero, so the head starts as an identity map on $x_t$. No rigid-body
projection or explicit cross-keypoint attention is applied.


\subsection{Training Objective}
\label{supp:kiva_training}

\paragraph{Forward process and objective.}
The corruption process and the training loss summarized in the main text are
\begin{equation}\label{eq:noise}
 x_t=\sqrt{\bar\alpha(t)}\,x_0+\sqrt{1-\bar\alpha(t)}\,\epsilon,
 \qquad
 \hat x_0=g_\theta(x_t,t,\mathcal F),
 \qquad
 \epsilon\sim\mathcal N(0,I),
\end{equation}
\begin{equation}\label{eq:loss}
 \mathcal L_{\mathrm{kp}}
 =\frac{1}{|\Omega|}\sum_{i\in\Omega}
 H_\beta\!\left(\hat x_{0,i}-x_{0,i}\right),
\end{equation}
where $\bar\alpha(t)\in(0,1]$ is the retained-signal schedule
($\bar\alpha\!\to\!1$ gives an almost clean input, $\bar\alpha\!\to\!0$ pure
noise), $g_\theta$ is the denoiser of Eq.~\eqref{eq:head}, $\Omega$ is the set
of valid scalar coordinates in the batch, and $H_\beta$ is the normalized Huber
penalty defined below. The model predicts the clean signal $\hat x_0$ rather
than the noise $\epsilon$.

\paragraph{Noise construction.}
For each training window we sample one noise level
$t\sim\mathcal U(10^{-4},1)$, shared across its frames and keypoints, and
independent Gaussian noise for every coordinate. The retained signal follows a
clipped cosine schedule:
\begin{equation}
\bar\alpha(t)=
\operatorname{clip}_{[10^{-5},1]}
\left[
\frac{\cos^2\!\left(\frac{t+s}{1+s}\frac{\pi}{2}\right)}
{\cos^2\!\left(\frac{s}{1+s}\frac{\pi}{2}\right)}
\right],
\qquad s=0.008,
\end{equation}
with $s$ a small offset preventing $\bar\alpha(0)$ from being degenerate.
Noisy inputs are constructed using Eq.~\eqref{eq:noise}. Noise levels and
Gaussian noise are resampled during training, with no additional loss weighting
by noise level.

\paragraph{Huber penalty.}
The normalized Huber penalty in Eq.~\eqref{eq:loss} is
\begin{equation}
H_\beta(\delta)=
\begin{cases}
\delta^2/(2\beta), & |\delta|<\beta,\\
|\delta|-\beta/2, & \text{otherwise},
\end{cases}
\end{equation}
so it is quadratic for small residuals and linear for large ones, limiting the
influence of outliers. This convention, also called smooth-L1, equals the
conventional Huber penalty divided by $\beta$. The transition parameter is
\begin{equation}
\beta=\frac{0.05}{\bar s},
\qquad
\bar s=\frac{1}{3}\sum_{c=1}^{3}\frac{h_c-\ell_c}{2},
\end{equation}
where $\bar s$ is the mean workspace half-span in meters and $h_c,\ell_c$ are
the box bounds on axis $c$. Because residuals are measured in normalized units,
$\beta$ corresponds to roughly $5$\,cm of metric error; for an anisotropic
workspace it does not correspond to exactly $5$\,cm on every axis.

\paragraph{Valid-coordinate averaging.}
The set $\Omega$ in Eq.~\eqref{eq:loss} contains every coordinate of every
keypoint in valid frames, excluding padding. Let $m_{b\tau}\in\{0,1\}$ indicate
whether frame $\tau$ in training window $b$ is valid. For a batch containing at
least one valid frame, the loss is equivalently
\begin{equation}
\mathcal L_{\mathrm{kp}}
=
\frac{
\sum_{b,\tau}m_{b\tau}
\sum_{k=1}^{K}\sum_{c=1}^{3}
H_\beta\!\left(\hat x_{0,b\tau kc}-x_{0,b\tau kc}\right)}
{3K\sum_{b,\tau}m_{b\tau}},
\end{equation}
where $K$ is the number of keypoints and $c$ indexes coordinate axes, so
$|\Omega|=3K\sum_{b,\tau}m_{b\tau}$. Windows with more valid frames contribute
proportionally more terms. The implementation replaces the valid-frame count in
the denominator with $\max(\sum_{b,\tau}m_{b\tau},10^{-8})$ to avoid division by
zero.

Only the diffusion head is optimized; the encoder stays frozen. No bone-length
or temporal-smoothness penalties are added, so the objective does not explicitly
enforce the properties subsequently assessed by the detectors.

\paragraph{Training windows and validation.}
Training uses batches of 32 windows, each containing 16 frames; shorter
sequences are padded and masked. Training and validation are split by scene,
keeping episodes from the same scene in the same split. Checkpoint selection
uses validation keypoint RMSE in metric coordinates, evaluated with the sampling
procedure in Appendix~\ref{supp:kiva_sampling}.


\subsection{Inference and Sampling}
\label{supp:kiva_sampling}

\paragraph{DDIM updates.}
Each sampling run starts from $x^{(0)}\sim\mathcal N(0,I)$ and performs ten DDIM
updates on a linearly spaced grid $t_0=1>\cdots>t_{10}=10^{-4}$. Writing
$\alpha_i=\bar\alpha(t_i)$, the update for $i=0,\ldots,9$ is
\begin{equation}
\begin{aligned}
\tilde x_0^{(i)}
&=\operatorname{clip}_{[-1,1]}g_\theta(x^{(i)},t_i,\mathcal F),\\
\hat\epsilon^{(i)}
&=\frac{x^{(i)}-\sqrt{\alpha_i}\,\tilde x_0^{(i)}}
{\max(\sqrt{1-\alpha_i},10^{-4})},\\
x^{(i+1)}
&=\sqrt{\alpha_{i+1}}\,\tilde x_0^{(i)}
+\sqrt{1-\alpha_{i+1}}\,\hat\epsilon^{(i)},
\end{aligned}
\end{equation}
where $\tilde x_0^{(i)}$ is the current clean-signal estimate, clipped to the
normalized workspace range, and $\hat\epsilon^{(i)}$ the implied noise estimate.
Visual features remain fixed throughout sampling. No fresh noise is injected
during the updates, making each trajectory deterministic once its initial noise
is fixed.

\paragraph{Final prediction and averaging.}
After the tenth update we make one additional clean-coordinate prediction at
$t_{10}$. For sampling run $n$,
\begin{equation}
\hat x_0^{(n)}
=\operatorname{clip}_{[-1,1]}
g_\theta(x^{(10,n)},t_{10},\mathcal F).
\end{equation}
We average five independently initialized runs and convert the result to metric
coordinates with the inverse workspace map of Eq.~\eqref{eq:supp-norm}:
\begin{equation}
P=E^{-1}\!\left(\frac{1}{5}\sum_{n=1}^{5}\hat x_0^{(n)}\right).
\end{equation}
Because $E^{-1}$ is affine, averaging before or after inverse normalization
gives the same result.

\paragraph{Cost.}
Each run requires eleven denoiser evaluations (ten DDIM updates plus the final
clean prediction), i.e.\ $55$ head evaluations per window. DINOv3 features are
encoded once and reused across all steps, samples, and noise levels.

\paragraph{Long videos.}
The reader processes non-overlapping windows of at most 64 frames and
concatenates their predicted trajectories. Temporal attention is bidirectional
within each window, so the reader operates offline. Attention does not cross
window boundaries.


\subsection{Detector and Calibration Conventions}
\label{supp:kiva_detectors}

\paragraph{Rigid keypoint pairs.}
The set $\mathcal B$ in Eq.~\eqref{eq:detectors} contains nondegenerate keypoint
pairs $(a,b)$ whose separation is fixed by the robot geometry. Nominal distances
$L_{ab}$ come from the robot description. Pairs whose distance changes with
joint articulation or gripper motion are excluded, preventing ordinary robot
movement from being counted as a rigidity violation.

\paragraph{Jerk and temporal boundaries.}
Jerk is computed on the concatenated trajectory using the frame interval
$\Delta t$ in seconds; the stencil $P_\tau-3P_{\tau-1}+3P_{\tau-2}-P_{\tau-3}$
is the third-order backward difference. The first three entries of each clip are
set to zero because the required history is unavailable. Subsequent differences
may cross reader-window boundaries, where discontinuities can affect the jerk
score. Division by $\Delta t^3$ gives physical units but does not eliminate
sensitivity to sampling rate or keypoint estimation noise.

\paragraph{Segment aggregation.}
Frames are grouped into non-overlapping segments $\mathcal S_i$ of $16$ frames.
Each segment yields one raw measurement per detector,
\begin{equation}\label{eq:supp-seg}
v_i^{\mathrm{rig}}=\operatorname{median}_{\tau\in\mathcal S_i}r_\tau,
\qquad
v_i^{\mathrm{jerk}}=\max_{\tau\in\mathcal S_i}j_\tau,
\end{equation}
with $r_\tau$ and $j_\tau$ from Eq.~\eqref{eq:detectors}. The median is used for
rigidity because an incorrect link length is a persistent rather than impulsive
violation, whereas the maximum is used for jerk because a single teleporting
frame is exactly the failure to expose.

\paragraph{Normalization by real-video thresholds.}
Let $\mathcal C_{\mathrm{real}}$ be a pool of calibration segments drawn from
real robot videos and processed by the identical pipeline (same reader, same
sampling, same segment length). For detector
$d\in\{\mathrm{rig},\mathrm{jerk}\}$,
\begin{equation}\label{eq:supp-calib}
\vartheta_d=Q_{0.95}\!\left(\{v_j^d:j\in\mathcal C_{\mathrm{real}}\}\right),
\qquad
s_i^d=\frac{v_i^d}{\vartheta_d},
\end{equation}
where $Q_{0.95}$ denotes the empirical $95$th percentile and $\vartheta_d>0$ is
assumed. Each detector is calibrated separately, using the same segment
statistics as evaluation. The score $s_i^d$ is dimensionless: $s_i^d=2$ means
the raw measurement is twice the real-video threshold, and is \emph{not} a
probability of physical invalidity.

The empirical $95$th-percentile threshold yields an approximately $5\%$
exceedance rate on the calibration segments, subject to finite-sample and tie
effects. It does not guarantee the same rate on unseen videos.

\paragraph{Measurement limitations.}
KIVA operates on predicted keypoints rather than directly observed 3D
trajectories. Reader errors can introduce apparent violations, while learned
priors, temporal context, and sample averaging can suppress genuine anomalies.
The scores therefore depend on the accuracy of the visual reader.
