# Supplementary material for: RoboWorM: Evaluating Movement Realism, Consistency and Acceleration Affects in Embodied Video World Models
Source: arXiv:2610.33807 source file (2026-10-24)
Supplement: Supplementary file 3 [file 8_llm.tex]

\section{The Use of Large Language Models}\label{supp:llm}
All scientific contributions, including the proposed method, experimental design, results, and analyses, are solely our own work. We made minimal use of large language models, specifically ChatGPT and Claude, solely to assist with paper presentation, including:

\begin{enumerate}[label=(\roman*)]
\item formatting tables and figures in \LaTeX, strictly for presentation purposes, and
\item refining sentence structure to improve clarity and readability.
\end{enumerate}
