# Supplementary material for: RoboWorM: Evaluating Movement Realism, Consistency and Acceleration Affects in Embodied Video World Models
Source: arXiv:2610.33807 source file (2026-10-24)
Supplement: Supplementary file 4 [file accel_by_config.tex]

% Generated by assets/scripts/make_accel_config_table.py -- do not edit by hand.
% Numbers are PLACEHOLDERS until a scoring wave is joined in.
% needs: longtable, booktabs, makecell, xcolor, cleveref, xspace
\providecommand{\ph}{\textcolor{black!30}{$\cdot$}}   % unfilled number
\providecommand{\na}{\texttt{--}}                      % not run / not measured

{\scriptsize
\setlength{\tabcolsep}{3.5pt}
\begin{longtable}{@{}lllrrrrrr@{}}
\caption{\textbf{Per-configuration results on \ours.} One row per (model, camera track, embodiment) configuration that exists in the benchmark, for the dense baseline and for every acceleration method. Values are \emph{absolute} medians over the clips of that configuration, each with a bootstrap CI, exactly as a reference-free benchmark column is normally reported; \textbf{Dense} is the reference row of its own configuration and every method below it is read against the dense row \emph{in the same configuration}, never across configurations. \emph{Speedup} is the measured wall-clock ratio of that configuration against its dense run. \texttt{--} marks a configuration the method was not run on, or one whose timing was not instrumented; it is never back-filled from another cell. $n$ is the largest per-metric clip count in the row. Absolute Active Motion Continuity is \emph{not} comparable across embodiments (humanoid sits well below the manipulators), which is precisely why this table is split by embodiment instead of pooling them. Ctrl-World is multi-view only and DreamDojo single-view only, hence one track each; Ctrl-World's 3-view and 4-view-grid multi-view layouts are pooled into one line. SiTo and ITM were not run on DreamDojo.}
\label{tab:supp_accel_by_config} \\
\toprule
\multicolumn{3}{@{}l}{Configuration} & & \multicolumn{4}{c}{Absolute median (reference-free)} & \\
\cmidrule(lr){5-8}
Model & Track & Embodiment & Speedup & \makecell{Visual\\Integrity} & \makecell{Actor\\Activity} & \makecell{Active\\Rate} & \makecell{Active Motion\\Continuity} & $n$ \\
\midrule
\endfirsthead
\multicolumn{9}{@{}l}{\emph{\cref{tab:supp_accel_by_config} continued from the previous page.}} \\
\toprule
\multicolumn{3}{@{}l}{Configuration} & & \multicolumn{4}{c}{Absolute median (reference-free)} & \\
\cmidrule(lr){5-8}
Model & Track & Embodiment & Speedup & \makecell{Visual\\Integrity} & \makecell{Actor\\Activity} & \makecell{Active\\Rate} & \makecell{Active Motion\\Continuity} & $n$ \\
\midrule
\endhead
\midrule
\multicolumn{9}{r@{}}{\emph{continued on the next page}} \\
\endfoot
\bottomrule
\endlastfoot
\multicolumn{9}{@{}l}{\textbf{Dense} \textit{(no acceleration)}} \\
\addlinespace[1pt]
Ctrl-World & multi-view & single-arm & 1.00$\times$ & \ph & \ph & \ph & \ph & \ph \\
 &  & bimanual & 1.00$\times$ & \ph & \ph & \ph & \ph & \ph \\
 &  & humanoid & 1.00$\times$ & \ph & \ph & \ph & \ph & \ph \\
\cmidrule(lr){1-3}
DreamGen & multi-view & single-arm & 1.00$\times$ & \ph & \ph & \ph & \ph & \ph \\
 &  & bimanual & 1.00$\times$ & \ph & \ph & \ph & \ph & \ph \\
 &  & humanoid & 1.00$\times$ & \ph & \ph & \ph & \ph & \ph \\
\cmidrule(lr){1-3}
DreamGen & single-view & single-arm & 1.00$\times$ & \ph & \ph & \ph & \ph & \ph \\
 &  & bimanual & 1.00$\times$ & \ph & \ph & \ph & \ph & \ph \\
 &  & humanoid & 1.00$\times$ & \ph & \ph & \ph & \ph & \ph \\
\cmidrule(lr){1-3}
DreamDojo & single-view & single-arm & 1.00$\times$ & \ph & \ph & \ph & \ph & \ph \\
 &  & bimanual & 1.00$\times$ & \ph & \ph & \ph & \ph & \ph \\
 &  & humanoid & 1.00$\times$ & \ph & \ph & \ph & \ph & \ph \\
\midrule
\multicolumn{9}{@{}l}{\textbf{DiCache} \textit{(step caching)}} \\
\addlinespace[1pt]
Ctrl-World & multi-view & single-arm & \ph & \ph & \ph & \ph & \ph & \ph \\
 &  & bimanual & \ph & \ph & \ph & \ph & \ph & \ph \\
 &  & humanoid & \ph & \ph & \ph & \ph & \ph & \ph \\
\cmidrule(lr){1-3}
DreamGen & multi-view & single-arm & \ph & \ph & \ph & \ph & \ph & \ph \\
 &  & bimanual & \ph & \ph & \ph & \ph & \ph & \ph \\
 &  & humanoid & \ph & \ph & \ph & \ph & \ph & \ph \\
\cmidrule(lr){1-3}
DreamGen & single-view & single-arm & \ph & \ph & \ph & \ph & \ph & \ph \\
 &  & bimanual & \ph & \ph & \ph & \ph & \ph & \ph \\
 &  & humanoid & \ph & \ph & \ph & \ph & \ph & \ph \\
\cmidrule(lr){1-3}
DreamDojo & single-view & single-arm & \ph & \ph & \ph & \ph & \ph & \ph \\
 &  & bimanual & \ph & \ph & \ph & \ph & \ph & \ph \\
 &  & humanoid & \ph & \ph & \ph & \ph & \ph & \ph \\
\midrule
\multicolumn{9}{@{}l}{\textbf{WorldCache} \textit{(step caching)}} \\
\addlinespace[1pt]
Ctrl-World & multi-view & single-arm & \ph & \ph & \ph & \ph & \ph & \ph \\
 &  & bimanual & \ph & \ph & \ph & \ph & \ph & \ph \\
 &  & humanoid & \ph & \ph & \ph & \ph & \ph & \ph \\
\cmidrule(lr){1-3}
DreamGen & multi-view & single-arm & \ph & \ph & \ph & \ph & \ph & \ph \\
 &  & bimanual & \ph & \ph & \ph & \ph & \ph & \ph \\
 &  & humanoid & \ph & \ph & \ph & \ph & \ph & \ph \\
\cmidrule(lr){1-3}
DreamGen & single-view & single-arm & \ph & \ph & \ph & \ph & \ph & \ph \\
 &  & bimanual & \ph & \ph & \ph & \ph & \ph & \ph \\
 &  & humanoid & \ph & \ph & \ph & \ph & \ph & \ph \\
\cmidrule(lr){1-3}
DreamDojo & single-view & single-arm & \ph & \ph & \ph & \ph & \ph & \ph \\
 &  & bimanual & \ph & \ph & \ph & \ph & \ph & \ph \\
 &  & humanoid & \ph & \ph & \ph & \ph & \ph & \ph \\
\midrule
\multicolumn{9}{@{}l}{\textbf{FasterCache} \textit{(step caching)}} \\
\addlinespace[1pt]
Ctrl-World & multi-view & single-arm & \ph & \ph & \ph & \ph & \ph & \ph \\
 &  & bimanual & \ph & \ph & \ph & \ph & \ph & \ph \\
 &  & humanoid & \ph & \ph & \ph & \ph & \ph & \ph \\
\cmidrule(lr){1-3}
DreamGen & multi-view & single-arm & \ph & \ph & \ph & \ph & \ph & \ph \\
 &  & bimanual & \ph & \ph & \ph & \ph & \ph & \ph \\
 &  & humanoid & \ph & \ph & \ph & \ph & \ph & \ph \\
\cmidrule(lr){1-3}
DreamGen & single-view & single-arm & \ph & \ph & \ph & \ph & \ph & \ph \\
 &  & bimanual & \ph & \ph & \ph & \ph & \ph & \ph \\
 &  & humanoid & \ph & \ph & \ph & \ph & \ph & \ph \\
\cmidrule(lr){1-3}
DreamDojo & single-view & single-arm & \ph & \ph & \ph & \ph & \ph & \ph \\
 &  & bimanual & \ph & \ph & \ph & \ph & \ph & \ph \\
 &  & humanoid & \ph & \ph & \ph & \ph & \ph & \ph \\
\midrule
\multicolumn{9}{@{}l}{\textbf{PISA} \textit{(sparse attention)}} \\
\addlinespace[1pt]
Ctrl-World & multi-view & single-arm & \ph & \ph & \ph & \ph & \ph & \ph \\
 &  & bimanual & \ph & \ph & \ph & \ph & \ph & \ph \\
 &  & humanoid & \ph & \ph & \ph & \ph & \ph & \ph \\
\cmidrule(lr){1-3}
DreamGen & multi-view & single-arm & \ph & \ph & \ph & \ph & \ph & \ph \\
 &  & bimanual & \ph & \ph & \ph & \ph & \ph & \ph \\
 &  & humanoid & \ph & \ph & \ph & \ph & \ph & \ph \\
\cmidrule(lr){1-3}
DreamGen & single-view & single-arm & \ph & \ph & \ph & \ph & \ph & \ph \\
 &  & bimanual & \ph & \ph & \ph & \ph & \ph & \ph \\
 &  & humanoid & \ph & \ph & \ph & \ph & \ph & \ph \\
\cmidrule(lr){1-3}
DreamDojo & single-view & single-arm & \ph & \ph & \ph & \ph & \ph & \ph \\
 &  & bimanual & \ph & \ph & \ph & \ph & \ph & \ph \\
 &  & humanoid & \ph & \ph & \ph & \ph & \ph & \ph \\
\midrule
\multicolumn{9}{@{}l}{\textbf{Radial} \textit{(sparse attention)}} \\
\addlinespace[1pt]
Ctrl-World & multi-view & single-arm & \ph & \ph & \ph & \ph & \ph & \ph \\
 &  & bimanual & \ph & \ph & \ph & \ph & \ph & \ph \\
 &  & humanoid & \ph & \ph & \ph & \ph & \ph & \ph \\
\cmidrule(lr){1-3}
DreamGen & multi-view & single-arm & \ph & \ph & \ph & \ph & \ph & \ph \\
 &  & bimanual & \ph & \ph & \ph & \ph & \ph & \ph \\
 &  & humanoid & \ph & \ph & \ph & \ph & \ph & \ph \\
\cmidrule(lr){1-3}
DreamGen & single-view & single-arm & \ph & \ph & \ph & \ph & \ph & \ph \\
 &  & bimanual & \ph & \ph & \ph & \ph & \ph & \ph \\
 &  & humanoid & \ph & \ph & \ph & \ph & \ph & \ph \\
\cmidrule(lr){1-3}
DreamDojo & single-view & single-arm & \ph & \ph & \ph & \ph & \ph & \ph \\
 &  & bimanual & \ph & \ph & \ph & \ph & \ph & \ph \\
 &  & humanoid & \ph & \ph & \ph & \ph & \ph & \ph \\
\midrule
\multicolumn{9}{@{}l}{\textbf{SVG1} \textit{(sparse attention)}} \\
\addlinespace[1pt]
Ctrl-World & multi-view & single-arm & \ph & \ph & \ph & \ph & \ph & \ph \\
 &  & bimanual & \ph & \ph & \ph & \ph & \ph & \ph \\
 &  & humanoid & \ph & \ph & \ph & \ph & \ph & \ph \\
\cmidrule(lr){1-3}
DreamGen & multi-view & single-arm & \ph & \ph & \ph & \ph & \ph & \ph \\
 &  & bimanual & \ph & \ph & \ph & \ph & \ph & \ph \\
 &  & humanoid & \ph & \ph & \ph & \ph & \ph & \ph \\
\cmidrule(lr){1-3}
DreamGen & single-view & single-arm & \ph & \ph & \ph & \ph & \ph & \ph \\
 &  & bimanual & \ph & \ph & \ph & \ph & \ph & \ph \\
 &  & humanoid & \ph & \ph & \ph & \ph & \ph & \ph \\
\cmidrule(lr){1-3}
DreamDojo & single-view & single-arm & \ph & \ph & \ph & \ph & \ph & \ph \\
 &  & bimanual & \ph & \ph & \ph & \ph & \ph & \ph \\
 &  & humanoid & \ph & \ph & \ph & \ph & \ph & \ph \\
\midrule
\multicolumn{9}{@{}l}{\textbf{SVG2} \textit{(sparse attention)}} \\
\addlinespace[1pt]
Ctrl-World & multi-view & single-arm & \ph & \ph & \ph & \ph & \ph & \ph \\
 &  & bimanual & \ph & \ph & \ph & \ph & \ph & \ph \\
 &  & humanoid & \ph & \ph & \ph & \ph & \ph & \ph \\
\cmidrule(lr){1-3}
DreamGen & multi-view & single-arm & \ph & \ph & \ph & \ph & \ph & \ph \\
 &  & bimanual & \ph & \ph & \ph & \ph & \ph & \ph \\
 &  & humanoid & \ph & \ph & \ph & \ph & \ph & \ph \\
\cmidrule(lr){1-3}
DreamGen & single-view & single-arm & \ph & \ph & \ph & \ph & \ph & \ph \\
 &  & bimanual & \ph & \ph & \ph & \ph & \ph & \ph \\
 &  & humanoid & \ph & \ph & \ph & \ph & \ph & \ph \\
\cmidrule(lr){1-3}
DreamDojo & single-view & single-arm & \ph & \ph & \ph & \ph & \ph & \ph \\
 &  & bimanual & \ph & \ph & \ph & \ph & \ph & \ph \\
 &  & humanoid & \ph & \ph & \ph & \ph & \ph & \ph \\
\midrule
\multicolumn{9}{@{}l}{\textbf{SiTo} \textit{(token pruning)}} \\
\addlinespace[1pt]
Ctrl-World & multi-view & single-arm & \ph & \ph & \ph & \ph & \ph & \ph \\
 &  & bimanual & \ph & \ph & \ph & \ph & \ph & \ph \\
 &  & humanoid & \ph & \ph & \ph & \ph & \ph & \ph \\
\cmidrule(lr){1-3}
DreamGen & multi-view & single-arm & \ph & \ph & \ph & \ph & \ph & \ph \\
 &  & bimanual & \ph & \ph & \ph & \ph & \ph & \ph \\
 &  & humanoid & \ph & \ph & \ph & \ph & \ph & \ph \\
\cmidrule(lr){1-3}
DreamGen & single-view & single-arm & \ph & \ph & \ph & \ph & \ph & \ph \\
 &  & bimanual & \ph & \ph & \ph & \ph & \ph & \ph \\
 &  & humanoid & \ph & \ph & \ph & \ph & \ph & \ph \\
\cmidrule(lr){1-3}
DreamDojo & single-view & single-arm & \na & \na & \na & \na & \na & \na \\
 &  & bimanual & \na & \na & \na & \na & \na & \na \\
 &  & humanoid & \na & \na & \na & \na & \na & \na \\
\midrule
\multicolumn{9}{@{}l}{\textbf{ITM} \textit{(token pruning)}} \\
\addlinespace[1pt]
Ctrl-World & multi-view & single-arm & \ph & \ph & \ph & \ph & \ph & \ph \\
 &  & bimanual & \ph & \ph & \ph & \ph & \ph & \ph \\
 &  & humanoid & \ph & \ph & \ph & \ph & \ph & \ph \\
\cmidrule(lr){1-3}
DreamGen & multi-view & single-arm & \ph & \ph & \ph & \ph & \ph & \ph \\
 &  & bimanual & \ph & \ph & \ph & \ph & \ph & \ph \\
 &  & humanoid & \ph & \ph & \ph & \ph & \ph & \ph \\
\cmidrule(lr){1-3}
DreamGen & single-view & single-arm & \ph & \ph & \ph & \ph & \ph & \ph \\
 &  & bimanual & \ph & \ph & \ph & \ph & \ph & \ph \\
 &  & humanoid & \ph & \ph & \ph & \ph & \ph & \ph \\
\cmidrule(lr){1-3}
DreamDojo & single-view & single-arm & \na & \na & \na & \na & \na & \na \\
 &  & bimanual & \na & \na & \na & \na & \na & \na \\
 &  & humanoid & \na & \na & \na & \na & \na & \na \\
\end{longtable}
}
