# Supplementary material for: RoboWorM: Evaluating Movement Realism, Consistency and Acceleration Affects in Embodied Video World Models
Source: arXiv:2610.33807 source file (2026-10-24)
Supplement: Supplementary file 5 [file accel_by_config_paired.tex]

% Generated by assets/scripts/make_accel_config_table.py -- do not edit by hand.
% Numbers are PLACEHOLDERS until a scoring wave is joined in.
% needs: longtable, booktabs, makecell, xcolor, cleveref, xspace
\providecommand{\ph}{\textcolor{black!30}{$\cdot$}}   % unfilled number
\providecommand{\na}{\texttt{--}}                      % not run / not measured

{\scriptsize
\setlength{\tabcolsep}{3.5pt}
\begin{longtable}{@{}lllrrrrrrr@{}}
\caption{\textbf{Per-configuration acceleration results on \ours.} The same configurations, reported as a \emph{paired} median delta against that configuration's own dense clip (accelerated $-$ dense, same episode, same matched frame grid): negative is worse than dense, and the value carries no absolute level, so a per-embodiment level difference cannot leak in. \emph{Speedup} is the measured wall-clock ratio of that same configuration. \texttt{--} marks a configuration the method was not run on, or one whose timing was not instrumented. $n$ is the largest per-metric pair count in the row. $^{*}$~resolved (bootstrap CI excludes $0$, Wilcoxon $p<0.05$, $n\ge8$); $^{\dagger}$~a solid move in a direction that cannot be an improvement (over-smoothing inflating Active Motion Continuity); $^{\sim}$~$n<8$, shown but not claimed. Ctrl-World is multi-view only and DreamDojo single-view only; SiTo and ITM were not run on DreamDojo.}
\label{tab:supp_accel_by_config_paired} \\
\toprule
\multicolumn{3}{@{}l}{Configuration} & & \multicolumn{5}{c}{Paired $\Delta$ vs.\ dense} & \\
\cmidrule(lr){5-9}
Model & Track & Embodiment & Speedup & \makecell{Visual\\Integrity} & \makecell{Text\\Align.} & \makecell{Actor\\Activity} & \makecell{Active\\Rate} & \makecell{Active Motion\\Continuity} & $n$ \\
\midrule
\endfirsthead
\multicolumn{10}{@{}l}{\emph{\cref{tab:supp_accel_by_config_paired} continued from the previous page.}} \\
\toprule
\multicolumn{3}{@{}l}{Configuration} & & \multicolumn{5}{c}{Paired $\Delta$ vs.\ dense} & \\
\cmidrule(lr){5-9}
Model & Track & Embodiment & Speedup & \makecell{Visual\\Integrity} & \makecell{Text\\Align.} & \makecell{Actor\\Activity} & \makecell{Active\\Rate} & \makecell{Active Motion\\Continuity} & $n$ \\
\midrule
\endhead
\midrule
\multicolumn{10}{r@{}}{\emph{continued on the next page}} \\
\endfoot
\bottomrule
\endlastfoot
\multicolumn{10}{@{}l}{\textbf{DiCache} \textit{(step caching)}} \\
\addlinespace[1pt]
Ctrl-World & multi-view & single-arm & \ph & \ph & \ph & \ph & \ph & \ph & \ph \\
 &  & bimanual & \ph & \ph & \ph & \ph & \ph & \ph & \ph \\
 &  & humanoid & \ph & \ph & \ph & \ph & \ph & \ph & \ph \\
\cmidrule(lr){1-3}
DreamGen & multi-view & single-arm & \ph & \ph & \ph & \ph & \ph & \ph & \ph \\
 &  & bimanual & \ph & \ph & \ph & \ph & \ph & \ph & \ph \\
 &  & humanoid & \ph & \ph & \ph & \ph & \ph & \ph & \ph \\
\cmidrule(lr){1-3}
DreamGen & single-view & single-arm & \ph & \ph & \ph & \ph & \ph & \ph & \ph \\
 &  & bimanual & \ph & \ph & \ph & \ph & \ph & \ph & \ph \\
 &  & humanoid & \ph & \ph & \ph & \ph & \ph & \ph & \ph \\
\cmidrule(lr){1-3}
DreamDojo & single-view & single-arm & \ph & \ph & \ph & \ph & \ph & \ph & \ph \\
 &  & bimanual & \ph & \ph & \ph & \ph & \ph & \ph & \ph \\
 &  & humanoid & \ph & \ph & \ph & \ph & \ph & \ph & \ph \\
\midrule
\multicolumn{10}{@{}l}{\textbf{WorldCache} \textit{(step caching)}} \\
\addlinespace[1pt]
Ctrl-World & multi-view & single-arm & \ph & \ph & \ph & \ph & \ph & \ph & \ph \\
 &  & bimanual & \ph & \ph & \ph & \ph & \ph & \ph & \ph \\
 &  & humanoid & \ph & \ph & \ph & \ph & \ph & \ph & \ph \\
\cmidrule(lr){1-3}
DreamGen & multi-view & single-arm & \ph & \ph & \ph & \ph & \ph & \ph & \ph \\
 &  & bimanual & \ph & \ph & \ph & \ph & \ph & \ph & \ph \\
 &  & humanoid & \ph & \ph & \ph & \ph & \ph & \ph & \ph \\
\cmidrule(lr){1-3}
DreamGen & single-view & single-arm & \ph & \ph & \ph & \ph & \ph & \ph & \ph \\
 &  & bimanual & \ph & \ph & \ph & \ph & \ph & \ph & \ph \\
 &  & humanoid & \ph & \ph & \ph & \ph & \ph & \ph & \ph \\
\cmidrule(lr){1-3}
DreamDojo & single-view & single-arm & \ph & \ph & \ph & \ph & \ph & \ph & \ph \\
 &  & bimanual & \ph & \ph & \ph & \ph & \ph & \ph & \ph \\
 &  & humanoid & \ph & \ph & \ph & \ph & \ph & \ph & \ph \\
\midrule
\multicolumn{10}{@{}l}{\textbf{FasterCache} \textit{(step caching)}} \\
\addlinespace[1pt]
Ctrl-World & multi-view & single-arm & \ph & \ph & \ph & \ph & \ph & \ph & \ph \\
 &  & bimanual & \ph & \ph & \ph & \ph & \ph & \ph & \ph \\
 &  & humanoid & \ph & \ph & \ph & \ph & \ph & \ph & \ph \\
\cmidrule(lr){1-3}
DreamGen & multi-view & single-arm & \ph & \ph & \ph & \ph & \ph & \ph & \ph \\
 &  & bimanual & \ph & \ph & \ph & \ph & \ph & \ph & \ph \\
 &  & humanoid & \ph & \ph & \ph & \ph & \ph & \ph & \ph \\
\cmidrule(lr){1-3}
DreamGen & single-view & single-arm & \ph & \ph & \ph & \ph & \ph & \ph & \ph \\
 &  & bimanual & \ph & \ph & \ph & \ph & \ph & \ph & \ph \\
 &  & humanoid & \ph & \ph & \ph & \ph & \ph & \ph & \ph \\
\cmidrule(lr){1-3}
DreamDojo & single-view & single-arm & \ph & \ph & \ph & \ph & \ph & \ph & \ph \\
 &  & bimanual & \ph & \ph & \ph & \ph & \ph & \ph & \ph \\
 &  & humanoid & \ph & \ph & \ph & \ph & \ph & \ph & \ph \\
\midrule
\multicolumn{10}{@{}l}{\textbf{PISA} \textit{(sparse attention)}} \\
\addlinespace[1pt]
Ctrl-World & multi-view & single-arm & \ph & \ph & \ph & \ph & \ph & \ph & \ph \\
 &  & bimanual & \ph & \ph & \ph & \ph & \ph & \ph & \ph \\
 &  & humanoid & \ph & \ph & \ph & \ph & \ph & \ph & \ph \\
\cmidrule(lr){1-3}
DreamGen & multi-view & single-arm & \ph & \ph & \ph & \ph & \ph & \ph & \ph \\
 &  & bimanual & \ph & \ph & \ph & \ph & \ph & \ph & \ph \\
 &  & humanoid & \ph & \ph & \ph & \ph & \ph & \ph & \ph \\
\cmidrule(lr){1-3}
DreamGen & single-view & single-arm & \ph & \ph & \ph & \ph & \ph & \ph & \ph \\
 &  & bimanual & \ph & \ph & \ph & \ph & \ph & \ph & \ph \\
 &  & humanoid & \ph & \ph & \ph & \ph & \ph & \ph & \ph \\
\cmidrule(lr){1-3}
DreamDojo & single-view & single-arm & \ph & \ph & \ph & \ph & \ph & \ph & \ph \\
 &  & bimanual & \ph & \ph & \ph & \ph & \ph & \ph & \ph \\
 &  & humanoid & \ph & \ph & \ph & \ph & \ph & \ph & \ph \\
\midrule
\multicolumn{10}{@{}l}{\textbf{Radial} \textit{(sparse attention)}} \\
\addlinespace[1pt]
Ctrl-World & multi-view & single-arm & \ph & \ph & \ph & \ph & \ph & \ph & \ph \\
 &  & bimanual & \ph & \ph & \ph & \ph & \ph & \ph & \ph \\
 &  & humanoid & \ph & \ph & \ph & \ph & \ph & \ph & \ph \\
\cmidrule(lr){1-3}
DreamGen & multi-view & single-arm & \ph & \ph & \ph & \ph & \ph & \ph & \ph \\
 &  & bimanual & \ph & \ph & \ph & \ph & \ph & \ph & \ph \\
 &  & humanoid & \ph & \ph & \ph & \ph & \ph & \ph & \ph \\
\cmidrule(lr){1-3}
DreamGen & single-view & single-arm & \ph & \ph & \ph & \ph & \ph & \ph & \ph \\
 &  & bimanual & \ph & \ph & \ph & \ph & \ph & \ph & \ph \\
 &  & humanoid & \ph & \ph & \ph & \ph & \ph & \ph & \ph \\
\cmidrule(lr){1-3}
DreamDojo & single-view & single-arm & \ph & \ph & \ph & \ph & \ph & \ph & \ph \\
 &  & bimanual & \ph & \ph & \ph & \ph & \ph & \ph & \ph \\
 &  & humanoid & \ph & \ph & \ph & \ph & \ph & \ph & \ph \\
\midrule
\multicolumn{10}{@{}l}{\textbf{SVG1} \textit{(sparse attention)}} \\
\addlinespace[1pt]
Ctrl-World & multi-view & single-arm & \ph & \ph & \ph & \ph & \ph & \ph & \ph \\
 &  & bimanual & \ph & \ph & \ph & \ph & \ph & \ph & \ph \\
 &  & humanoid & \ph & \ph & \ph & \ph & \ph & \ph & \ph \\
\cmidrule(lr){1-3}
DreamGen & multi-view & single-arm & \ph & \ph & \ph & \ph & \ph & \ph & \ph \\
 &  & bimanual & \ph & \ph & \ph & \ph & \ph & \ph & \ph \\
 &  & humanoid & \ph & \ph & \ph & \ph & \ph & \ph & \ph \\
\cmidrule(lr){1-3}
DreamGen & single-view & single-arm & \ph & \ph & \ph & \ph & \ph & \ph & \ph \\
 &  & bimanual & \ph & \ph & \ph & \ph & \ph & \ph & \ph \\
 &  & humanoid & \ph & \ph & \ph & \ph & \ph & \ph & \ph \\
\cmidrule(lr){1-3}
DreamDojo & single-view & single-arm & \ph & \ph & \ph & \ph & \ph & \ph & \ph \\
 &  & bimanual & \ph & \ph & \ph & \ph & \ph & \ph & \ph \\
 &  & humanoid & \ph & \ph & \ph & \ph & \ph & \ph & \ph \\
\midrule
\multicolumn{10}{@{}l}{\textbf{SVG2} \textit{(sparse attention)}} \\
\addlinespace[1pt]
Ctrl-World & multi-view & single-arm & \ph & \ph & \ph & \ph & \ph & \ph & \ph \\
 &  & bimanual & \ph & \ph & \ph & \ph & \ph & \ph & \ph \\
 &  & humanoid & \ph & \ph & \ph & \ph & \ph & \ph & \ph \\
\cmidrule(lr){1-3}
DreamGen & multi-view & single-arm & \ph & \ph & \ph & \ph & \ph & \ph & \ph \\
 &  & bimanual & \ph & \ph & \ph & \ph & \ph & \ph & \ph \\
 &  & humanoid & \ph & \ph & \ph & \ph & \ph & \ph & \ph \\
\cmidrule(lr){1-3}
DreamGen & single-view & single-arm & \ph & \ph & \ph & \ph & \ph & \ph & \ph \\
 &  & bimanual & \ph & \ph & \ph & \ph & \ph & \ph & \ph \\
 &  & humanoid & \ph & \ph & \ph & \ph & \ph & \ph & \ph \\
\cmidrule(lr){1-3}
DreamDojo & single-view & single-arm & \ph & \ph & \ph & \ph & \ph & \ph & \ph \\
 &  & bimanual & \ph & \ph & \ph & \ph & \ph & \ph & \ph \\
 &  & humanoid & \ph & \ph & \ph & \ph & \ph & \ph & \ph \\
\midrule
\multicolumn{10}{@{}l}{\textbf{SiTo} \textit{(token pruning)}} \\
\addlinespace[1pt]
Ctrl-World & multi-view & single-arm & \ph & \ph & \ph & \ph & \ph & \ph & \ph \\
 &  & bimanual & \ph & \ph & \ph & \ph & \ph & \ph & \ph \\
 &  & humanoid & \ph & \ph & \ph & \ph & \ph & \ph & \ph \\
\cmidrule(lr){1-3}
DreamGen & multi-view & single-arm & \ph & \ph & \ph & \ph & \ph & \ph & \ph \\
 &  & bimanual & \ph & \ph & \ph & \ph & \ph & \ph & \ph \\
 &  & humanoid & \ph & \ph & \ph & \ph & \ph & \ph & \ph \\
\cmidrule(lr){1-3}
DreamGen & single-view & single-arm & \ph & \ph & \ph & \ph & \ph & \ph & \ph \\
 &  & bimanual & \ph & \ph & \ph & \ph & \ph & \ph & \ph \\
 &  & humanoid & \ph & \ph & \ph & \ph & \ph & \ph & \ph \\
\cmidrule(lr){1-3}
DreamDojo & single-view & single-arm & \na & \na & \na & \na & \na & \na & \na \\
 &  & bimanual & \na & \na & \na & \na & \na & \na & \na \\
 &  & humanoid & \na & \na & \na & \na & \na & \na & \na \\
\midrule
\multicolumn{10}{@{}l}{\textbf{ITM} \textit{(token pruning)}} \\
\addlinespace[1pt]
Ctrl-World & multi-view & single-arm & \ph & \ph & \ph & \ph & \ph & \ph & \ph \\
 &  & bimanual & \ph & \ph & \ph & \ph & \ph & \ph & \ph \\
 &  & humanoid & \ph & \ph & \ph & \ph & \ph & \ph & \ph \\
\cmidrule(lr){1-3}
DreamGen & multi-view & single-arm & \ph & \ph & \ph & \ph & \ph & \ph & \ph \\
 &  & bimanual & \ph & \ph & \ph & \ph & \ph & \ph & \ph \\
 &  & humanoid & \ph & \ph & \ph & \ph & \ph & \ph & \ph \\
\cmidrule(lr){1-3}
DreamGen & single-view & single-arm & \ph & \ph & \ph & \ph & \ph & \ph & \ph \\
 &  & bimanual & \ph & \ph & \ph & \ph & \ph & \ph & \ph \\
 &  & humanoid & \ph & \ph & \ph & \ph & \ph & \ph & \ph \\
\cmidrule(lr){1-3}
DreamDojo & single-view & single-arm & \na & \na & \na & \na & \na & \na & \na \\
 &  & bimanual & \na & \na & \na & \na & \na & \na & \na \\
 &  & humanoid & \na & \na & \na & \na & \na & \na & \na \\
\end{longtable}
}
