# Supplementary material for: RoboWorM: Evaluating Movement Realism, Consistency and Acceleration Affects in Embodied Video World Models
Source: arXiv:2610.33807 source file (2026-10-24)
Supplement: Supplementary file 6 [file fig_accel_taxonomy.tex]

% ============================================================================
%  PLACEHOLDER -- REPLACE WITH A HAND-DRAWN SCHEMATIC
% ============================================================================
%  Export the drawing to:  assets/paper/figures/fig_accel_taxonomy.pdf
%  Then delete the \fbox{...} placeholder block below and uncomment the
%  \includegraphics line. Nothing else needs to change; the caption, label and
%  the \cref{fig:supp_accel_taxonomy} references in 3_implemetation_details.tex
%  are already wired up.
%
%  WHAT THE DRAWING SHOULD SHOW
%  ----------------------------
%  One denoising step, left to right, with the three method families annotated
%  at the exact point each one intervenes. The purpose is to make visible that
%  they attack *different* costs, which is what explains why their speedups do
%  not compose and why each family wins on a different backbone.
%
%   [x_t, action/text cond.]
%        |
%        v
%   +--------------------------------------------------+
%   |  transformer / U-Net block  (x L blocks)         |
%   |                                                  |
%   |   tokens --> [ SELF-ATTENTION ] --> [ CROSS ] --> [ MLP ]
%   |                    ^                                     |
%   +--------------------|-------------------------------------+
%        |               |
%        v               |
%   [ scheduler step ] --+
%        |
%        v
%   [x_{t-1}]  --> ... --> [VAE decode] --> frames
%
%  Annotate three interventions, ideally in three distinct colours matching the
%  figures (token reduction #e76f51, caching #2a9d8f, sparse attention #c1121f):
%
%  (1) TOKEN REDUCTION (SiTo, ITM) -- a bracket on the *token sequence entering*
%      the attention op. Show N tokens being merged/pruned to kN before
%      attention and un-merged after. Mark that on the Ctrl-World U-Net this
%      reaches only the *spatial* attention, not the temporal attention, which
%      is why its ceiling there is ~1.08x (see fig_time_budget panel b).
%
%  (2) CACHING (WorldCache, DiCache, FasterCache) -- an arrow that *skips the
%      whole block stack* for a subset of scheduler steps, reusing the previous
%      step's residual. Draw the step axis (t = T..0) with a few steps struck
%      through, and mark the leading "warm-up" steps that are always computed
%      densely (the ret_ratio knob). This is the only family that reduces the
%      *number* of forward passes rather than the cost of one.
%
%  (3) SPARSE ATTENTION (PISA, SVG, SVG2, Radial) -- a QK^T attention matrix
%      with only some blocks shaded, sitting *inside* the self-attention box.
%      Emphasise that it shrinks one operator, so its ceiling is bounded by that
%      operator's share of runtime -- the Amdahl argument of the prose.
%
%  A small inset showing the measured self-attention share per backbone (27%
%  DreamGen, 15-18% DreamDojo, 7% Ctrl-World spatial) would tie the schematic to
%  fig_time_budget, but is optional -- that figure already carries the numbers.
% ============================================================================
\begin{figure}[t]
\centering
% --- Uncomment once the drawing has been exported: -------------------------
% \includegraphics[width=\linewidth]{figures/fig_accel_taxonomy.pdf}
% --- Delete everything from here to the marker below: ----------------------
\fbox{\begin{minipage}[c][0.30\textheight][c]{0.965\linewidth}
\centering
\textsc{placeholder}\\[0.6em]
{\normalsize\bfseries Hand-drawn schematic pending}\\[0.9em]
\begin{minipage}{0.86\linewidth}\small\raggedright
A single denoising step, annotated with the point at which each method family
intervenes: \textbf{token reduction} on the token sequence entering attention,
\textbf{step caching} skipping whole block stacks across scheduler steps, and
\textbf{sparse attention} inside the $QK^{\top}$ operator. See the comment block
at the top of \texttt{appendix/figures/fig\_accel\_taxonomy.tex} for the full
drawing brief.
\end{minipage}
\end{minipage}}
% --- to here. ---------------------------------------------------------------
\caption{\textbf{Where each acceleration family intervenes in one denoising
step.} The three families reduce three different costs, which is why their
speedups are not interchangeable across backbones. \emph{Token reduction}
(SiTo, ITM) shrinks the token sequence entering attention and restores it
afterwards; on the Ctrl-World U-Net it reaches only the spatial attention, never
the temporal attention, which bounds it near $1.08\times$
(Fig.~\ref{fig:supp_time_budget}b). \emph{Step caching} (WorldCache, DiCache,
FasterCache) is the only family that reduces the \emph{number} of network
evaluations rather than the cost of one: it reuses a previous step's residual and
skips whole block stacks, after a leading warm-up fraction that is always
computed densely. \emph{Sparse attention} (PISA, SVG, SVG2, Radial) shrinks a
single operator, so its attainable speedup is capped by that operator's share of
runtime --- the Amdahl bound of Fig.~\ref{fig:supp_time_budget}b, which is what
explains the negative sparse-attention results in this benchmark.}
\label{fig:supp_accel_taxonomy}
\end{figure}
